# Supplementary material for: Zero-Shot Heterogeneous Transfer Learning from Recommender Systems to Cold-Start Search Retrieval
Source: arXiv:2008.02930 source file (2020-08-19)
Supplement: Supplementary file 1 [file supp.tex]

%!TEX root = main.tex

\section{Supplement}
TODO
